# Supplementary material for: On the electronic path integral normal modes of the Meyer-Miller-Stock-Thoss representation of nonadiabatic dynamics
Source: arXiv:2508.14775 ancillary file (2025-10-06)
Supplement: Supplementary file 1 [file SI_electronic_normal_modes_arxiv.pdf]

# Supplementary Material: On the electronic normal modes of the Meyer–Miller–Stock–Thoss representation of non-adiabatic dynamics

Lauren E. Cook[1] and Timothy J. H. Hele[1, a)]

*Department of Chemistry, University College London, Christopher Ingold Building, London WC1H 0AJ, United Kingdom*

(Dated: 20 August 2025)

Here, we provide additional algebra and figures for the investigation into Meyer–Miller–Stock–Thoss (MMST) electronic normal modes. In Section I, we provide the derivation of the correlation function (CF) used in the calculations, the partition function and sampling and proof that the CF should be real. In Section II, we show symmetric potential matrix results for the $C_{11}(t)$ correlation function, the conservation of the quantum Boltzmann distribution (QBD) and energy for a single trajectory and QBD conservation for an ensemble of trajectories. We present the convergence of the ensemble calculation with increasing number of trajectories for different truncations of beads/normal modes using the asymmetric potential tested in the main work. We also show distributions of alternative metrics based on MMST variables and normal modes of these, including electronic populations and populations of state 1, where we also find no constraint on the higher normal modes.

a)Electronic mail: t.hele@ucl.ac.uk

## I. SUPPLEMENTARY ALGEBRA

### A. Correlation Function Derivation

Here, we present the derivation of the CF in MMST variables from Eqn. (19) of the main manuscript. This is a similar derivation as to Refs. [1] and [2] but we only consider the electronic system here. We wish to derive the form of,

$$C_{AB}^{[N]}(t) = \frac{1}{(2\pi\hbar)^{FN}} \iint d\mathbf{q} d\mathbf{p} [e^{\beta_N \hat{H}} \hat{A}]_{\overline{W}} \times [\hat{B}(t)]_W, \tag{S.1}$$

in mapping variables where we sum over $F$ electronic states and $N$ beads and,

$$[\hat{B}(t)]_W = \prod_j^N \int d\boldsymbol{\mu}'_j e^{i\boldsymbol{\mu}'_j \mathbf{p}_j/\hbar} \left\langle \mathbf{q}_j + \boldsymbol{\mu}'_j/2 \right| e^{i\hat{H}t/\hbar} \hat{B} e^{-i\hat{H}t/\hbar} \left| \mathbf{q}_j - \boldsymbol{\mu}'_j/2 \right\rangle, \tag{S.2a}$$

$$[e^{-\beta_N \hat{H}} \hat{A}]_{\overline{W}} = \prod_j^N \int d\boldsymbol{\mu}_j \sum_{n_j, m_j} e^{i\boldsymbol{\mu}_j \mathbf{p}_j/\hbar} \left\langle \mathbf{q}_{j-1} - \boldsymbol{\mu}_{j-1}/2 | n_{j-1} \right\rangle$$
$$\times \left\langle n_{j-1} \right| \frac{1}{2}(\hat{A} e^{-\beta\hat{H}} + e^{-\beta\hat{H}} \hat{A}) \left| m_j \right\rangle \left\langle m_j | \mathbf{q}_j + \boldsymbol{\mu}_j/2 \right\rangle, \tag{S.2b}$$

and $\int d\mathbf{q} = \prod_j^N \int d\mathbf{q}_j$ and likewise for $\mathbf{p}$.[1,3] The operators are only evaluated once in the path-integral loop such that, $\hat{A} = 1/N(\sum_j^N \hat{A}_j)$ and likewise for $\hat{B}$.

#### 1. *Real-time Propagation*

Using creation and annihilation operators,

$$\hat{B} = \sum_{n,m} \hat{a}_n^\dagger B_{nm} \hat{a}_m = \frac{1}{2\hbar} \sum_{n,m} (\hat{q}_n \hat{q}_m + \hat{p}_n \hat{p}_m - \hbar \delta_{nm}) B_{nm}, \tag{S.3}$$

such that

$$[\hat{B}(t)]_W = \frac{1}{N} \sum_j^N \int d\boldsymbol{\mu}'_j e^{i\boldsymbol{\mu}'_j \mathbf{p}_j/\hbar} \left\langle \mathbf{q}_j + \boldsymbol{\mu}'_j/2 \right| e^{i\hat{H}t/\hbar} \hat{B}_j e^{-i\hat{H}t/\hbar} \left| \mathbf{q}_j - \boldsymbol{\mu}'_j/2 \right\rangle \tag{S.4a}$$
$$= \frac{1}{N} \sum_j^N \int d\boldsymbol{\mu}'_j e^{i\boldsymbol{\mu}'_j \mathbf{p}_j/\hbar} \left\langle \mathbf{q}_j + \boldsymbol{\mu}'_j/2 \right| e^{i\hat{H}t/\hbar}$$
$$\times \frac{1}{2\hbar} \sum_{n_j, m_j}^F (\hat{q}_{n_j} \hat{q}_{m_j} + \hat{p}_{n_j} \hat{p}_{m_j} - \hbar \delta_{nm}) B_{n_j m_j} e^{-i\hat{H}t/\hbar} \left| \mathbf{q}_j - \boldsymbol{\mu}'_j/2 \right\rangle, \tag{S.4b}$$

where $n_j$ and $m_j$ are the electronic state indices for the $j$-th bead such that there is a sum over the electronic states for each bead index. This can be split into three terms; position-only, momentum-only, and constant terms. All three of these are known to transform as themselves under the Wigner

transform such that,

$$[\hat{B}(t)]_W = \frac{1}{N}\sum_j^N \left( \frac{1}{2\hbar} \sum_{n_j m_j} \left( q_{n_j} q_{m_j} + p_{n_j} p_{m_j} + \hbar \delta_{n_j m_j} \right)(t) B_{n_j m_j} \right) \tag{S.5a}$$

$$= \frac{1}{2\hbar N} \sum_j^N \mathrm{Tr}\left[ (\mathbf{C}_j(t) - \hbar \mathbb{I}) \mathbf{B}_j \right], \tag{S.5b}$$

where $\mathbf{C}_j(t) = (\mathbf{q}_j + i\mathbf{p}_j)(t) \otimes (\mathbf{q}_j - i\mathbf{p}_j)^{\mathrm{T}}(t)$ and $\mathbf{B}_j$ is the operator matrix for that bead. Here, we have chosen to evolve the **C** matrix with time but an alternative option is to directly evolve the **B** matrix instead.[1]

### *2. Imaginary-time Propagation*

Letting $\mathscr{O} = \frac{1}{2}(\hat{A} e^{-\beta \hat{H}} + e^{-\beta \hat{H}} \hat{A})$ such that $\langle n_{j-1} | \mathscr{O} | m_j \rangle = \mathscr{O}^j_{n_{j-1} m_j}$ and where,

$$\left\langle \mathbf{q}_{j-1} - \boldsymbol{\mu}_{j-1}/2 | n_{j-1} \right\rangle = \sqrt{\frac{2}{\hbar}} \frac{1}{(\pi\hbar)^{F/4}} (\mathbf{q}_{j-1} - \boldsymbol{\mu}_{j-1}/2)^{\mathrm{T}}_{n_{j-1}} e^{-(\mathbf{q}_{j-1} - \boldsymbol{\mu}_{j-1}/2)^{\mathrm{T}} (\mathbf{q}_{j-1} - \boldsymbol{\mu}_{j-1}/2)/2\hbar}, \tag{S.6}$$

$$\left\langle m_j | \mathbf{q}_j + \boldsymbol{\mu}_j/2 \right\rangle = \sqrt{\frac{2}{\hbar}} \frac{1}{(\pi\hbar)^{F/4}} (\mathbf{q}_j + \boldsymbol{\mu}_j/2)_{m_j} e^{-(\mathbf{q}_j + \boldsymbol{\mu}_j/2)^{\mathrm{T}} (\mathbf{q}_j + \boldsymbol{\mu}_j/2)/2\hbar}, \tag{S.7}$$

The imaginary-time propagation in Eqn. (S.2b) becomes,

$$[e^{-\beta_N \hat{H}} \hat{A}]_{\overline{W}} = \prod_j^N \int d\boldsymbol{\mu}_j e^{i\boldsymbol{\mu}_j \mathbf{p}_j/\hbar} \frac{2}{\hbar (\pi\hbar)^{F/2}} e^{-(|\mathbf{q}_{j-1} - \boldsymbol{\mu}_{j-1}/2|^2/2\hbar)} e^{-(|\mathbf{q}_j + \boldsymbol{\mu}_j/2|^2/2\hbar)}$$
$$\times (\mathbf{q}_{j-1} - \boldsymbol{\mu}_{j-1}/2)^{\mathrm{T}} \mathscr{O} (\mathbf{q}_j + \boldsymbol{\mu}_j/2), \tag{S.8}$$

where the product of the exponents becomes $e^{-\sum_j (|\mathbf{q}_j|^2 + |\boldsymbol{\mu}_j/2|^2)/\hbar}$ such that,

$$[e^{-\beta_N \hat{H}} \hat{A}]_{\overline{W}} = \left(\frac{2}{\hbar}\right)^N \frac{1}{(\pi\hbar)^{FN/2}} e^{-\sum_j |\mathbf{q}_j|^2/\hbar} \int d\boldsymbol{\mu}/\hbar_{k\neq j}\, e^{\sum_{k\neq j} i\boldsymbol{\mu}_k \mathbf{p}_k/\hbar} e^{-\sum_{k\neq j} |\boldsymbol{\mu}_k/2|^2/\hbar}$$
$$\times \int d\boldsymbol{\mu}_j\, e^{i\boldsymbol{\mu}_j \mathbf{p}_j/\hbar} e^{-|\boldsymbol{\mu}_j/2|^2/\hbar} (\mathbf{q}_{j-1} - \boldsymbol{\mu}_{j-1}/2)^{\mathrm{T}} \mathscr{O}^j_{n_{j-1} m_j} (\mathbf{q}_j + \boldsymbol{\mu}_j/2)$$
$$\times \prod_{k=j+1}^{j} (\mathbf{q}_{k-1} - \boldsymbol{\mu}_{k-1}/2)^{\mathrm{T}} \mathscr{O}^k_{n_{k-1} m_k} (\mathbf{q}_k + \boldsymbol{\mu}_k/2)(\mathbf{q}_j - \boldsymbol{\mu}_j/2)^{\mathrm{T}} \mathscr{O}^{j+1}_{n_j m_{j+1}} (\mathbf{q}_{j+1} + \boldsymbol{\mu}_{j+1}/2), \tag{S.9}$$

which due to cyclic symmetry,

$$[e^{-\beta_N \hat{H}} \hat{A}]_{\overline{W}} = \left(\frac{2}{\hbar}\right)^N \frac{1}{(\pi\hbar)^{FN/2}} e^{-\sum_j |\mathbf{q}_j|^2/\hbar} \int d\boldsymbol{\mu}_{k\neq j}\, e^{\sum_{k\neq j} i\boldsymbol{\mu}_k \mathbf{p}_k/\hbar} e^{-\sum_{k\neq j} |\boldsymbol{\mu}_k/2|^2/\hbar}$$
$$\times \int d\boldsymbol{\mu}_j\, e^{i\boldsymbol{\mu}_j \mathbf{p}_j/\hbar} e^{-|\boldsymbol{\mu}_j/2|^2/\hbar} (\mathbf{q}_j - \boldsymbol{\mu}_j/2)^{\mathrm{T}} \mathbf{F}_j (\mathbf{q}_j + \boldsymbol{\mu}_j/2), \tag{S.10}$$

where,

$$\mathbf{F}_j = \mathscr{O}^j_{n_j m_{j+1}} (\mathbf{q}_{j+1} + \boldsymbol{\mu}_{j+1}/2) \prod_{k=j+2}^{j-1} (\mathbf{q}_{k-1} - \boldsymbol{\mu}_{k-1}/2)^{\mathrm{T}} \mathscr{O}^k_{n_{k-1} m_k} (\mathbf{q}_k + \boldsymbol{\mu}_k/2)$$
$$\times (\mathbf{q}_{j-1} - \boldsymbol{\mu}_{j-1}/2)^{\mathrm{T}} \mathscr{O}^{j+1}_{n_j m_{j+1}}, \tag{S.11}$$

is the matrix of all the remaining cross-bead terms. To simplify things, we consider the integral on the second line of Eqn. (S.10) such that,

$$I = \int d\boldsymbol{\mu}_j \, e^{i\boldsymbol{\mu}_j \mathbf{p}_j/\hbar} e^{-|\boldsymbol{\mu}_j/2|^2/\hbar} (\mathbf{q}_j - \boldsymbol{\mu}_j/2)^{\mathrm{T}} \mathbf{F}_j (\mathbf{q}_j + \boldsymbol{\mu}_j/2), \tag{S.12}$$

where the exponent can be expressed as,

$$e^{i\boldsymbol{\mu}_j \mathbf{p}_j/\hbar} e^{-|\boldsymbol{\mu}_j/2|^2/\hbar} = e^{-(\boldsymbol{\mu}_j - 2i\mathbf{p}_j)^{\mathrm{T}}(\boldsymbol{\mu}_j - 2i\mathbf{p}_j)/4\hbar} e^{-\mathbf{p}_j^{\mathrm{T}} \mathbf{p}_j/\hbar}, \tag{S.13}$$

and the second exponent not dependant on $\boldsymbol{\mu}$ can be brought outside the integral, such that,

$$I = e^{-\mathbf{p}_j^{\mathrm{T}} \mathbf{p}_j/\hbar} \int d\boldsymbol{\mu}_j e^{-(\boldsymbol{\mu}_j - 2i\mathbf{p}_j)^{\mathrm{T}}(\boldsymbol{\mu}_j - 2i\mathbf{p}_j)/4\hbar} (\mathbf{q}_j - \boldsymbol{\mu}_j/2)^{\mathrm{T}} \mathbf{F}_j (\mathbf{q}_j + \boldsymbol{\mu}_j/2), \tag{S.14}$$

we can perform contour integration with the variable change, $\boldsymbol{\mu}'_j = \boldsymbol{\mu}_j - 2i\mathbf{p}_j$,

$$I = e^{-\mathbf{p}_j^{\mathrm{T}} \mathbf{p}_j/\hbar} \int d\boldsymbol{\mu}_j e^{-|\boldsymbol{\mu}'_j|^2/4\hbar} (\mathbf{q}_j^{\mathrm{T}} \mathbf{F}_j \mathbf{q}_j + \mathbf{p}_j^{\mathrm{T}} \mathbf{F}_j \mathbf{p}_j - i\mathbf{p}_j^{\mathrm{T}} \mathbf{F}_j \mathbf{q}_j + i\mathbf{q}_j^{\mathrm{T}} \mathbf{F}_j \mathbf{p}_j - \boldsymbol{\mu}_j^{\mathrm{T}} \mathbf{F}_j \boldsymbol{\mu}_j/4), \tag{S.15}$$

where we evaluate standard Gaussian integrals, noting that odd integrals are zero such that,

$$I = \left(\sqrt{4\hbar\pi}\right)^F e^{-\mathbf{p}_j^{\mathrm{T}} \mathbf{p}_j/\hbar} \left( \sum_{n_j, m_j}^{f} q_{j,n_j} q_{j,m_j} + p_{j,n_j} p_{j,m_j} + i p_{j,n_j} q_{j,m_j} - i q_{j,n_j} p_{j,m_j} - \frac{\hbar}{2} \delta_{n_j m_j} \right) \mathbf{F}_{j,n_j m_j}, \tag{S.16}$$

As we know that,

$$\mathrm{Tr}[\mathbf{C}_j \mathbf{D}] = \sum_{n_j, m_j}^{f} \left( q_{j,n_j} q_{j,m_j} + p_{j,n_j} p_{j,m_j} + i p_{j,n_j} q_{j,m_j} - i q_{j,n_j} p_{j,m_j} \right) \mathbf{D}_{n_j, m_j}, \tag{S.17}$$

where the imaginary terms only cancel if the matrix $\mathbf{D}$ is symmetric (as utilized in the real-time propagation). Inserting this and repeating $N$ times,

$$[e^{-\beta_N \hat{H}} \hat{A}]_{\overline{W}} = \frac{2^{N(F+1)}}{\hbar^N} e^{-(\sum_j |\mathbf{q}_j|^2 + |\mathbf{p}_j|^2)/\hbar} \mathrm{Tr} \left[ \prod_j^N \mathscr{O}^j \left( \mathbf{C}_j - \frac{\hbar}{2} \mathbb{I} \right) \right], \tag{S.18}$$

we obtain the final form for the imaginary-time propagation which is similar to the decoupled-case in Ref. [2].[1]

## B. Partition Function and Sampling

The partition function is,

$$Z = \mathrm{Tr}\left[e^{-\beta\hat{H}}\right] = \mathrm{Tr}\left[\prod_j^N e^{-\beta_N\hat{H}}\right], \tag{S.19}$$

To derive this in mapping variables we can follow a similar derivation to the correlation function, using Wigner transforms to obtain,

$$\begin{aligned} Z = \prod_j^N \sum_{n_j,m_j}^F \int d\mathbf{q}_j d\boldsymbol{\mu}_j d\mathbf{p}_j \frac{1}{(2\pi\hbar)^F} e^{i\boldsymbol{\mu}_j\mathbf{p}_j/\hbar} \left\langle \mathbf{q}_{j-1} - \boldsymbol{\mu}_{j-1}/2 | n_{j-1} \right\rangle \\ \times \left\langle n_{j-1} \right| e^{-\beta_N\hat{H}} \left| m_j \right\rangle \left\langle m_j | \mathbf{q}_j + \boldsymbol{\mu}_j/2 \right\rangle. \end{aligned} \tag{S.20}$$

The same steps as in Section I A 2 can be followed such that,

$$Z = \left(\frac{2}{\hbar}\right)^N \frac{1}{(\hbar\pi)^{FN}} \iint d\mathbf{q}d\mathbf{p}\, e^{-\mathscr{G}_{\mathrm{tot}}/\hbar} \mathrm{Tr}\left[\prod_j^N e^{-\beta_N\hat{H}} \left(\mathbf{C}_j - \frac{\hbar}{2}\mathbb{I}\right)\right], \tag{S.21}$$

where $\mathscr{G}_{\mathrm{tot}} = \sum_j |\mathbf{q}_j|^2 + |\mathbf{p}_j|^2$. We can define a distribution,

$$\tilde{\rho} = \frac{1}{(\pi\hbar)^{FN}} e^{-\mathscr{G}_{\mathrm{tot}}/\hbar} \left| \mathrm{Tr}\left[\prod_j^N e^{-\beta_N\hat{H}} \left(\mathbf{C}_j - \frac{\hbar}{2}\mathbb{I}\right)\right] \right|, \tag{S.22}$$

that can be sampled using a Metropolis-Hastings algorithm, such that,

$$Z = \left(\frac{2}{\hbar}\right)^N \iint d\mathbf{q}d\mathbf{p}\, \tilde{\rho} \times \mathrm{sgn}\left(\mathrm{Tr}\left[\prod_j^N e^{-\beta_N\hat{H}} \left(\mathbf{C}_j - \frac{\hbar}{2}\mathbb{I}\right)\right]\right) \tag{S.23}$$

$$= \left(\frac{2}{\hbar}\right)^N \langle \mathrm{sgn}(W) \rangle_{\tilde{\rho}}, \tag{S.24}$$

where $W = \mathrm{Tr}\left[\prod_j^N e^{-\beta_N \hat{H}}\left(\mathbf{C}_j - \frac{\hbar}{2}\mathbb{I}\right)\right]$. The CF should be normalized within the partition function such that,

$$C_{AB}^{[N]}(t) = \frac{2^{N-1}}{Z\hbar^{N+1}(\pi\hbar)^{FN}N}\iint d\mathbf{q}d\mathbf{p}\; e^{-\mathscr{G}_{\mathrm{tot}}/\hbar}\mathrm{Tr}\left[\prod_j^N \mathscr{O}^j\left(\mathbf{C}_j - \frac{\hbar}{2}\mathbb{I}\right)\right]\sum_j^N \mathrm{Tr}\left[(\mathbf{C}_j - \hbar\mathbb{I})\mathbf{B}_j(t)\right] \tag{S.25}$$

$$= \frac{2^{N-1}}{Z\hbar^{N+1}N}\iint d\mathbf{q}d\mathbf{p}\;\tilde{\rho}\times\frac{\mathrm{Tr}\left[\prod_j^N \mathscr{O}^j\left(\mathbf{C}_j - \frac{\hbar}{2}\mathbb{I}\right)\right]}{|W|}\sum_j^N \mathrm{Tr}\left[(\mathbf{C}_j - \hbar\mathbb{I})\mathbf{B}_j(t)\right] \tag{S.26}$$

$$= \frac{2^{N-1}}{Z\hbar^{N+1}N}\left\langle\frac{\mathrm{Tr}\left[\prod_j^N \mathscr{O}^j\left(\mathbf{C}_j - \frac{\hbar}{2}\mathbb{I}\right)\right]}{|W|}\sum_j^N \mathrm{Tr}\left[(\mathbf{C}_j - \hbar\mathbb{I})\mathbf{B}_j(t)\right]\right\rangle_{\tilde{\rho}} \tag{S.27}$$

$$= \frac{1}{2\hbar N}\frac{\left\langle\frac{\mathrm{Tr}\left[\prod_j^N \mathscr{O}^j\left(\mathbf{C}_j - \frac{\hbar}{2}\mathbb{I}\right)\right]}{|W|}\sum_j^N \mathrm{Tr}\left[(\mathbf{C}_j - \hbar\mathbb{I})\mathbf{B}_j(t)\right]\right\rangle_{\tilde{\rho}}}{\langle \mathrm{sgn}(W)\rangle_{\tilde{\rho}}}, \tag{S.28}$$

where the in the limit of a large number of $J$ trajectories,

$$C_{AB}^{[N]}(t) = \frac{1}{2\hbar N}\frac{\sum_J\left\{\frac{\mathrm{Tr}\left[\prod_j^N \mathscr{O}^j\left(\mathbf{C}_j - \frac{\hbar}{2}\mathbb{I}\right)\right]}{|W|}\sum_j^N \mathrm{Tr}\left[(\mathbf{C}_j - \hbar\mathbb{I})\mathbf{B}_j(t)\right]\right\}}{\sum_J \mathrm{sgn}(W)}. \tag{S.29}$$

## C. Real Correlation Function Proof

Here, we prove that the CF should be real and any imaginary terms that arise can be ignored.

In general, we note that a function $f(x)$ is hermitian if $f(-x) = f^*(x)$ where the real-part is even and the imaginary part is odd, such that,

$$\int_{-L}^{L} f(x)\,dx = \text{real}\;\forall L \in \mathbb{R}, \tag{S.30}$$

hence,

$$\int_{-L}^{L} f(x)g(x)\,dx = \begin{cases} \text{real if } g(x) \text{ is even and real} \\ \text{imaginary if } g(x) \text{ is odd and real.} \end{cases} \tag{S.31}$$

For our CF,

$$C_{AB}(t) \propto \left\langle \mathrm{Tr}\left[\prod_j^N \mathscr{O}^j\left(\mathbf{C}_j - \frac{\hbar}{2}\mathbb{I}\right)\right]\times\prod_j^N \mathrm{Tr}\left[\left(\mathbf{C}_j - \hbar\mathbb{I}\right)\mathbf{B}(t)\right]\right\rangle_{\tilde{\rho}}, \tag{S.32}$$

which has real normalisation seen in Eqn. (S.29), we can define,

$$f(\mathbf{q},\mathbf{p}) = \mathrm{Tr}\left[\prod_{j}^{N}\mathscr{O}^{j}\left(\mathbf{C}_j - \frac{\hbar}{2}\mathbb{I}\right)\right], \tag{S.33a}$$

$$g(\mathbf{q},\mathbf{p}) = \prod_{j}^{N}\mathrm{Tr}\left[\left(\mathbf{C}_j(t) - \hbar\mathbb{I}\right)\mathbf{B}_j\right], \tag{S.33b}$$

such that when sampling enough phase-space this becomes of the same form as the integral in Eqn. (S.31). If we are able to show that $f(\mathbf{q},\mathbf{p})$ is hermitian and that $g(\mathbf{p})$ is real and even, this would be sufficient to show that the CF is real.

To prove that the $f(\mathbf{p})$ is hermitian, we take the complex conjugate as,

$$f^{*}(\mathbf{q},\mathbf{p}) = \mathrm{Tr}\left[\prod_{j}^{N}\mathscr{O}^{j}\left(\mathbf{C}^{*}_j(\mathbf{q},\mathbf{p}) - \frac{\hbar}{2}\mathbb{I}\right)\right] \tag{S.34a}$$

$$= \mathrm{Tr}\left[\prod_{j}^{N}\mathscr{O}^{j}\left(\mathbf{C}_j(\mathbf{q},-\mathbf{p}) - \frac{\hbar}{2}\mathbb{I}\right)\right], \tag{S.34b}$$

as $\mathbf{C}_j = (\mathbf{q}_j + i\mathbf{p}_j)\otimes(\mathbf{q}_j - i\mathbf{p}_j)^{\mathrm{T}}$. This means $f(\mathbf{q},\mathbf{p})$ is hermitian and odd with respect to $\mathbf{p}$.

For $g(\mathbf{q},\mathbf{p})$, we wish to show this is real and even. As we again have the $\mathbf{C}$ matrix, any odd terms with respect to $\mathbf{p}$ arise from the imaginary terms. For a $2\times 2$ matrix, the $j$-th bead becomes,

$$\sum_{n_j,m_j}(-i\mathbf{p}_{n_j}\mathbf{q}_{m_j} + i\mathbf{q}_{n_j}\mathbf{p}_{m_j})\mathbf{B}_{n_j,m_j} = (-i\mathbf{p}_1\mathbf{q}_2 + i\mathbf{q}_1\mathbf{p}_2)\mathbf{B}_{12} + (-i\mathbf{p}_2\mathbf{q}_1 + i\mathbf{q}_2\mathbf{p}_1)\mathbf{B}_{21} \tag{S.35a}$$

$$\begin{cases} = 0 & \mathbf{B}_{12} = \mathbf{B}_{21} \\ \neq 0 & \mathbf{B}_{12} \neq \mathbf{B}_{21}, \end{cases} \tag{S.35b}$$

such that, if the $\mathbf{B}$ operator is symmetric, which for us it is, then the imaginary terms cancel. Hence the sum over all beads will also have the imaginary terms cancelling such that the $g(\mathbf{q},\mathbf{p})$ is real and even.

This means that when sampling the whole phase space (such that we evaluate the integral) the CF will be real. Hence, for finite sampling, we can discard any imaginary terms that arise.

## II. SUPPLEMENTARY FIGURES

### A. Symmetric Potential Matrix

The results for a symmetric potential where, $\mathbf{V} = \left[\begin{smallmatrix} 0 & 1 \\ 1 & 0 \end{smallmatrix}\right]$ and $N = 8$ are presented below.

### *1. Autocorrelation Function*

The $C_{11}$ correlation function is shown in Figure S.1, where we have additionally included the 7 bead/normal mode calculation. As in the main work, we see that all 8 beads/normal modes are required to converge on the Kubo-Transformed result.

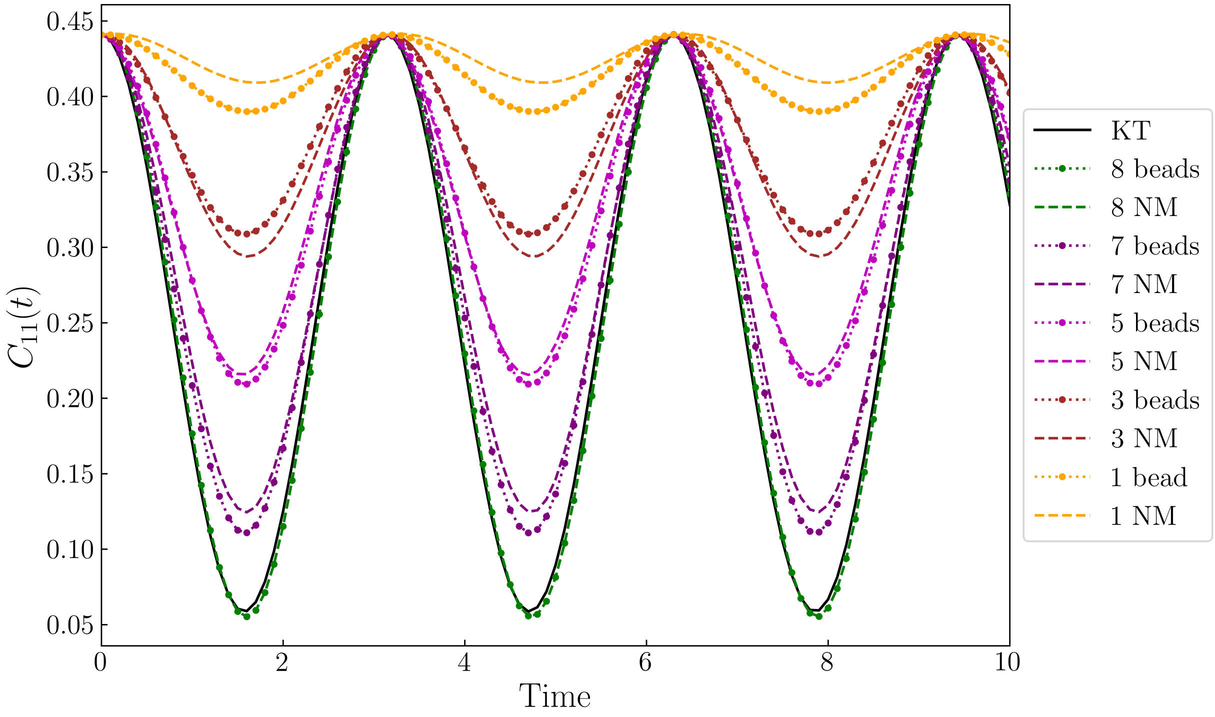


FIG. S.1. Correlation function for the electronic population of the first state with the exact Kubo-Transformed result (KT, black) compared with a full 8 bead calculation with truncation in both beads (dotted circle) and normal modes (NM, dashed) for; 8 (green), 7 (purple), 5 (magenta), 3 (red) and 1 (orange). It can be seen that while the result improves with more beads/normal modes included, all need to be included to converge on the correct answer

### *2. Quantum Boltzmann Distribution Conservation*

Figure S.2 shows the single trajectory conservation of the Boltzmann term and energy. Again, we see that these are only conserved for the full 8 bead/normal mode calculation.

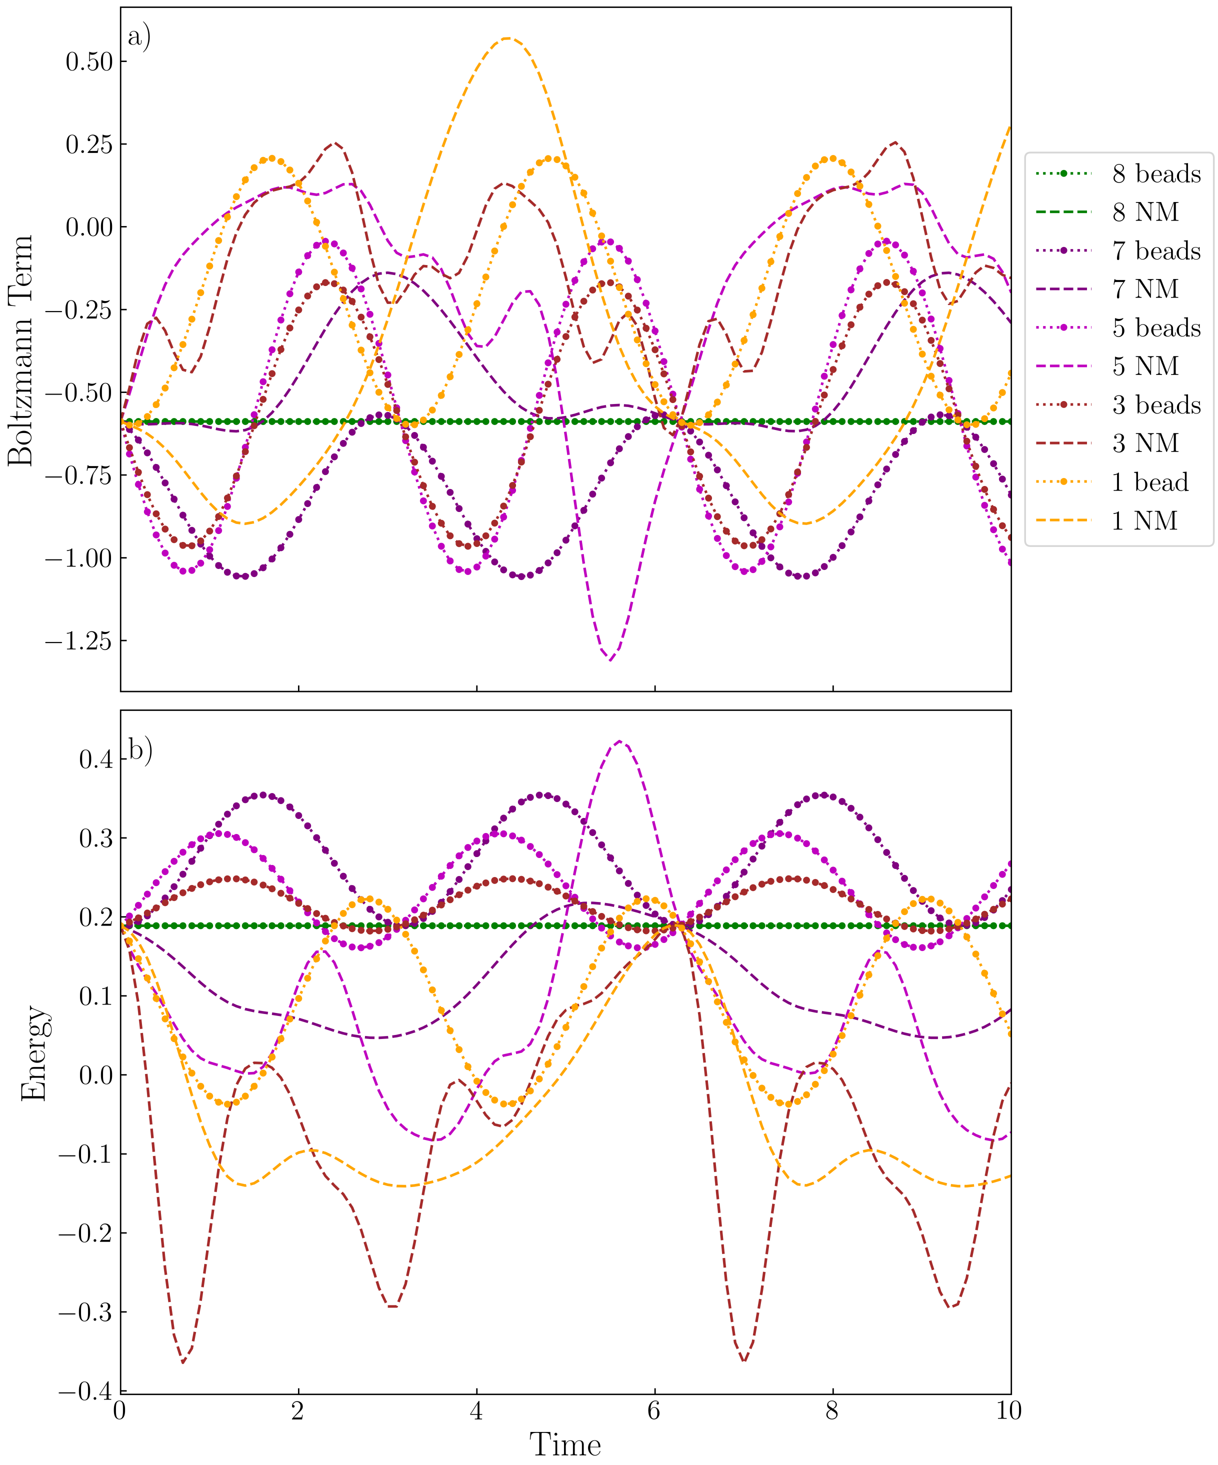


FIG. S.2. a) The propagated Boltzmann term and b) Energy against time for a single trajectory with a full 8 bead calculation with truncation in beads (dotted circle) and normal modes (dashed) for; 8 (green), 7 (purple), 5 (magenta), 3 (red) and 1 (orange). The 8 beads and normal modes are the only lines that are flat, indicating conserved QBD and energy.

The ensemble conservation of the QBD is in Figure S.3. The oscillations are slightly larger than the asymmetric results but still within 0.05 of the Kubo-Transformed result. Due to the Monte-Carlo sampling used, full convergence is challenging to obtain without a very large number of trajectories.

### 3. *QBD Conservation for Truncating in Beads/Normal Modes*

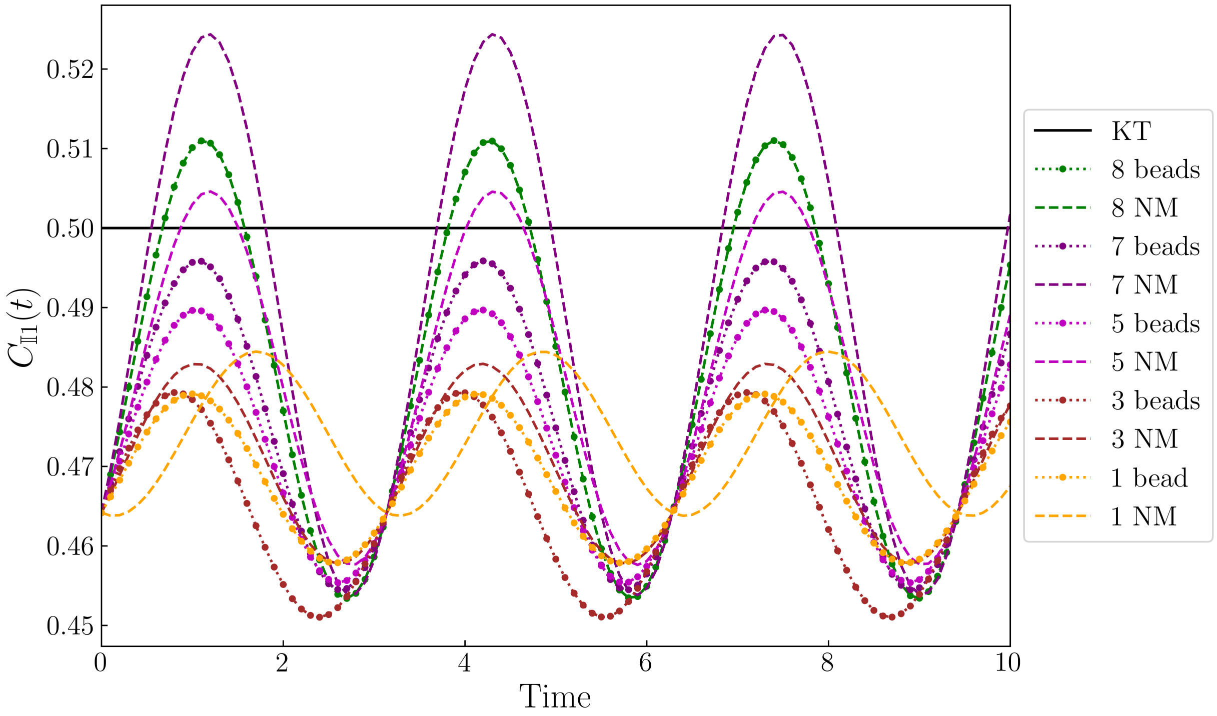


FIG. S.3. Correlation function for the conservation of electronic population of the first state with the exact Kubo-Transformed result (KT, black) compared with a full 8 bead calculation with truncation in both beads (dotted) and normal modes (NM, dashed) for; 8 (green), 5 (magenta), 3 (red) and 1 (orange). All oscillation are within 0.05 of the Kubo-Transformed result so there appears to be an averaging effect resulting in conservation.

## B. Asymmetric Potential

Additional results for the asymmetric potential, $\mathbf{V} = \left[\begin{smallmatrix} 1 & 1 \\ 1 & -1 \end{smallmatrix}\right]$ and $N = 8$ are presented below.

### 1. *Increasing Trajectory Convergence*

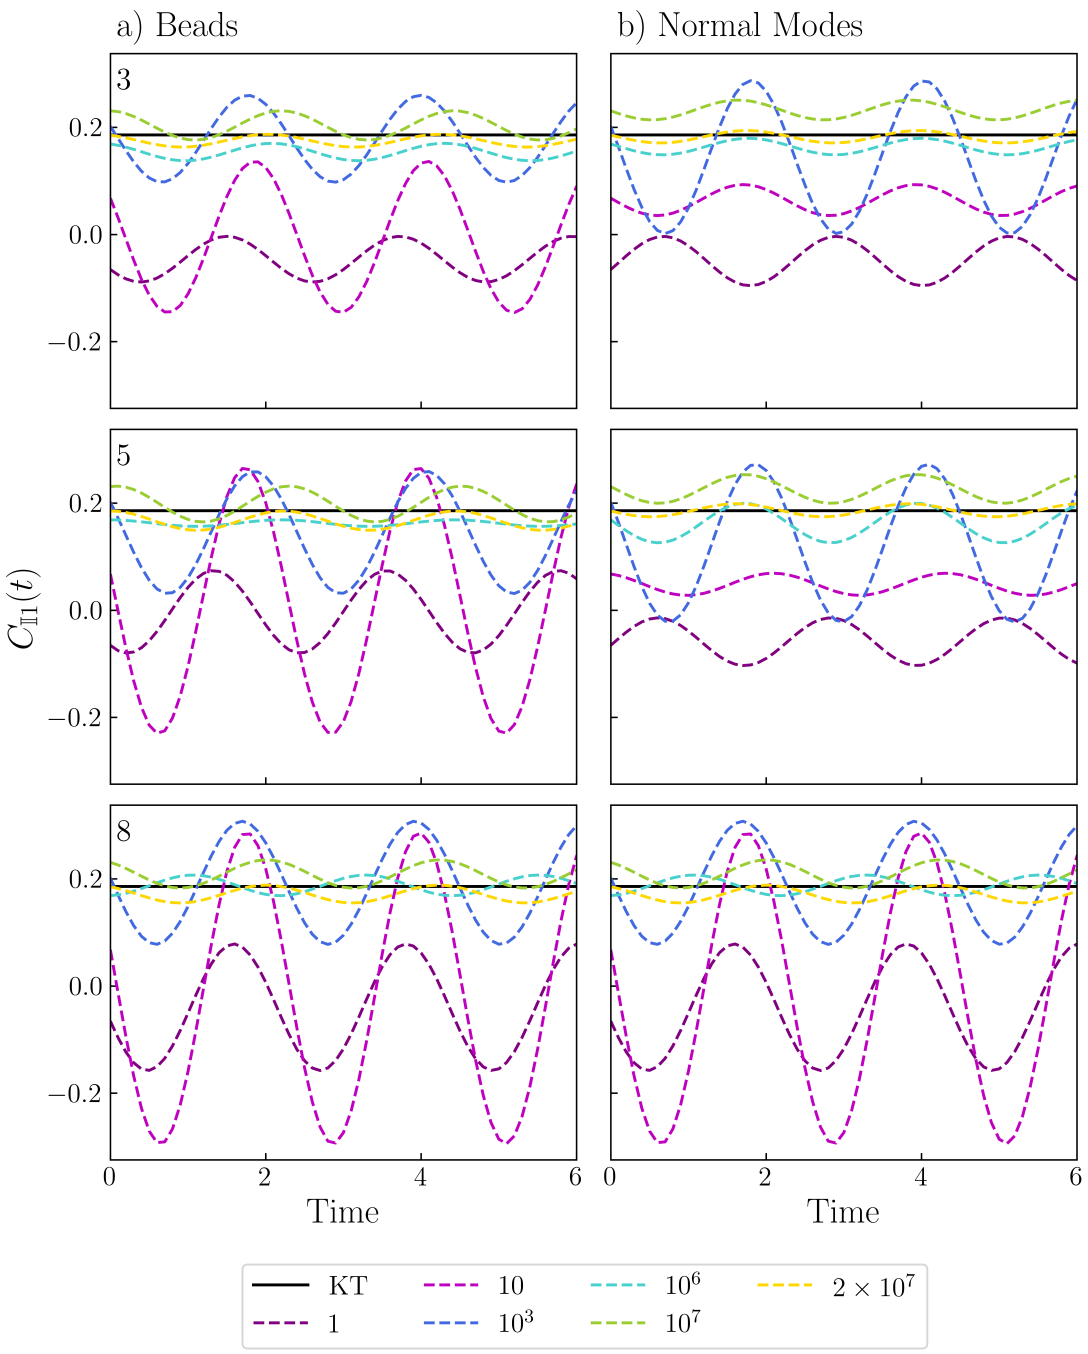


FIG. S.4. Correlation function for the conservation of electronic population of the first state with the exact Kubo-Transformed result (KT, black) compared with a full 4 bead calculation with different numbers of trajectories; 1 (purple), 10 (magenta), $10^3$ (blue), $10^5$ (light blue), $10^6$ (green) and $10^7$ (yellow). The beads (left) and normal modes (right) with truncation of 3 (top row), 5 (middle row) and full 8 (bottom row). A general trend is observed where increasing the number of trajectories improves the conservation for all truncations of beads/normal modes indicating an averaging effect.

In Figure S.4, we show the comparison increasing the number of trajectories for 3, 5 and 8 beads and normal modes for the asymmetric potential tested in the main work. We see that averaging over more trajectories improves the convergence of all truncations despite the fact that only the full 8 bead/normal mode calculations conserve the QBD for a single trajectory.

### 2. *Alternative Metric Distributions*

We additionally investigated alternative metrics based on MMST variables and took normal modes of these, to see if there are any constraints on the distributions using the asymmetric potential. Firstly we looked at the distributions of the total populations of each bead, calculated by evaluating Eqn. (32) from the main manuscript, and transformed this into normal modes. As seen in Figure S.5, we see that all bead populations have the same distribution. For the normal modes, only the lowest normal mode is centred around a non-zero value and the distribution standard deviations are very similar. This means that there does not appear to be any constraint on the higher normal modes when looking at the electronic population.

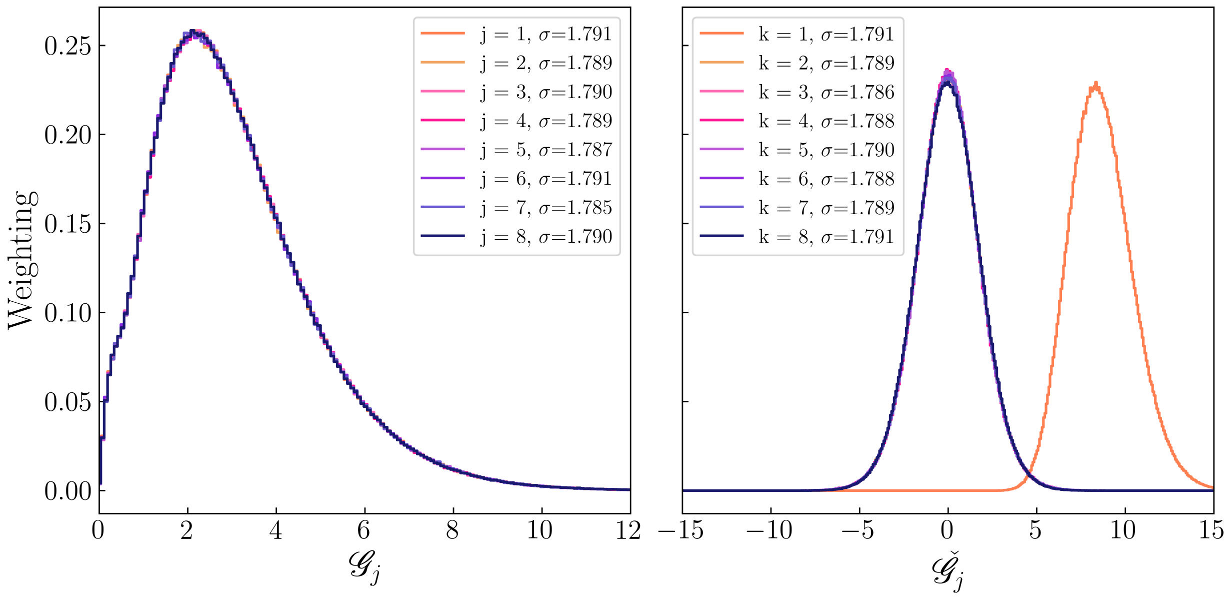


FIG. S.5. Histogram of the initial total electronic populations in beads (left plot) and normal modes (right plot) with the standard deviation of each in the legend. We see that all the beads have the same distribution, as expected. The normal modes of total population have very similar distributions and only the lowest normal mode is significantly populated such that there is no constraint on the higher normal modes.

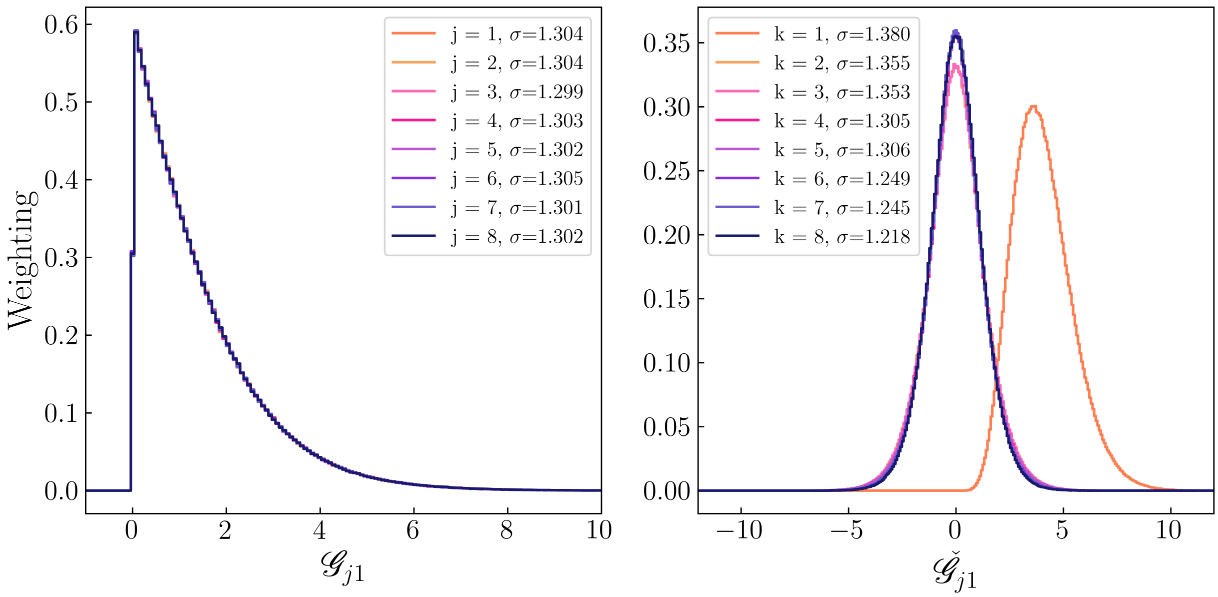


FIG. S.6. Histogram of the initial electronic population of state 1 in beads (left plot) and normal modes (right plot) with the standard deviation of each in the legend. All the beads have the same distribution, however, the centroid has a non-zero centred distribution compared with the higher modes.

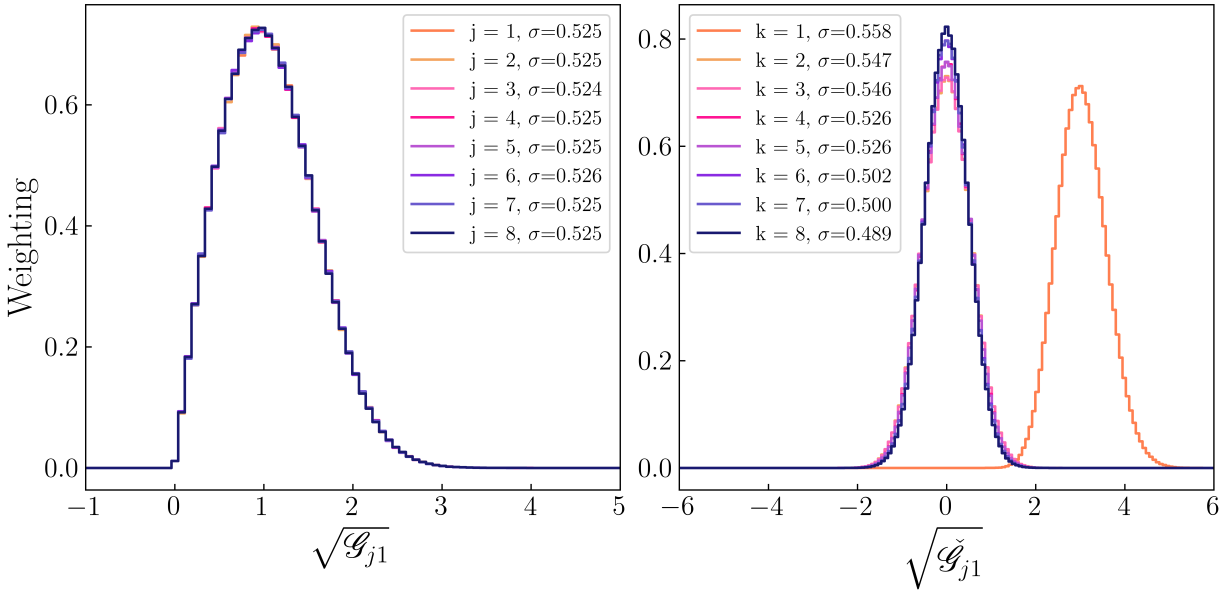


FIG. S.7. Histogram of the radius of the initial electronic population of state 1 in beads (left plot) and normal modes (right plot) with the standard deviation of each in the legend. This is similar to the population of state 1 plot above but the distributions are narrower.

We then investigated the first electronic state probability in beads, calculated as described earlier but not summing over both electronic states, and transformed into normal modes. This is similar to Figure S.5 but just for the first electronic state, Figure S.6. All the beads have the same distribution as we would expect. Again, only the lowest normal mode is centred around a non-zero value indicating that it has a higher population. From these we see a very slight narrowing of the higher normal modes but this is not very significant and the distributions are still very similar. Therefore, we find no constraint on the state populations either.

Lastly, we tested the radius of the state probability by taking the square root of the first electronic state probability and transformed this into normal modes. In Figure S.7, we see that the distributions are significantly narrower than for the state probability (Figure S.6) but show the same trends.

We conclude that to find a constraint on the normal modes, an alternative metric will need to be utilised instead of the normal modes of the MMST variables and of various electronic population metrics based on MMST variables. We intend to approach this in future work by considering what may give rise to a constraint in the electronic degrees of freedom, similar to how the springs between beads constrains the normal modes in the free ring-polymer.[3]

## REFERENCES


[1]T. J. Hele and N. Ananth, Faraday Discuss. **195**, 269 (2016).

[2]S. N. Chowdhury and P. Huo, J. Chem. Phys. **154**, 124124 (2021).

[3]T. J. H. Hele, M. J. Willatt, A. Muolo, and S. C. Althorpe, J. Chem. Phys. **142**, 134103 (2015).
